# Supplementary material for: Gaussian theory for estimating fluctuating perturbations with back action evasive oscillator variables
Source: arXiv:2202.13314 source file (2022-02-27)
Supplement: Supplementary file 3 [file preamble.tex]

\usepackage{graphicx}% Include figure files
\usepackage{dcolumn}% Align table columns on decimal point
\usepackage{bm}% bold math
\usepackage{bbm}% bold math
%\usepackage{hyperref}% add hypertext capabilities
%\usepackage[mathlines]{lineno}% Enable numbering of text and display math
%\linenumbers\relax % Commence numbering lines

\usepackage[pdftex,dvipsnames]{xcolor}
\usepackage{hyperref}
\hypersetup{frenchlinks = true,
	colorlinks,
	linkcolor={red!50!black},
	citecolor={blue!50!black},
	urlcolor={blue}
}

\usepackage{mathtools}
\usepackage{printlen}
\usepackage{enumitem}

\usepackage{siunitx}
\usepackage{stfloats}% <-- added for S
\usepackage{braket}
\usepackage{nicematrix}
%\usepackage[showframe,%Uncomment any one of the following lines to test 
%%scale=0.7, marginratio={1:1, 2:3}, ignoreall,% default settings
%%text={7in,10in},centering,
%%margin=1.5in,
%%total={6.5in,8.75in}, top=1.2in, left=0.9in, includefoot,
%%height=10in,a5paper,hmargin={3cm,0.8in},
%]{geometry}

\def\mat#1{\bm{#1}}
\def\op#1{\hat{#1}}
\def\vecop#1{\vec{\op{#1}}}
\renewcommand\vec{\bm}

\def\st#1{_{\mathrm{#1}}}
\def\ut#1{^{\mathrm{#1}}}

\renewcommand{\Re}{\mathrm{Re}}
\newcommand{\fig}[0]{Fig.~}
\newcommand{\dt}[0]{{\delta t}}
\newcommand{\I}{\mathbbm 1}
\renewcommand{\O}{\mathbb O}

\newcommand{\R}{\mathcal R}

\newcommand{\W}[0]{\mathcal W}
\newcommand{\tr}[0]{\mathrm{tr}}

\newcommand{\rhotop}[0]{\op{\tilde{\rho}}}

%\def\x#1{\op{x}\st{#1}}

\usepackage{ifthen}

\newcommand{\x}[1][]{%
	\ifthenelse{\equal{#1}{}}{\op x}{\op x_{#1}}%
}

\newcommand{\p}[1][]{%
	\ifthenelse{\equal{#1}{}}{\op p}{\op p_{#1}}%
}

\usepackage{xifthen}
%\renewcommand{\covar}[2]{%
\DeclareRobustCommand{\covar}[2]{ % this makes it work in captions
	%\ifthenelse{\equal{#1}{}}{\op p}{\op p_{#1}}%
	\ifthenelse{\equal{#1}{}}{\Delta {#2} ^2}{\Delta (#1, #2)}%
}

%\newcommand{\std}[2]{%
\DeclareRobustCommand{\std}[2]{%
	%\ifthenelse{\equal{#1}{}}{\op p}{\op p_{#1}}%
	\ifthenelse{\equal{#1}{}}{\Delta #2 }{\sqrt{\Delta (#1, #2)}}%
}

%\newcommand{\covar}[2]{\Delta (#1, #2)}

\renewcommand{\H}{\op H}

%%%%% ALGORITHM
\usepackage{algorithm}
\usepackage{algpseudocode}

%%%%%%%
\usepackage{graphicx}
\graphicspath{ {./figs/}{./figs/fig1/}{./figs/fig2/} } 
%%%%%%%
